# Supplementary material for: Winding Numbers and Topology of Aperiodic Tilings
Source: arXiv:2110.08798 source file (2021-10-17)
Supplement: Supplementary file 1 [file supplementary.pdf]

# Supplementary Material: Winding Numbers and Topology of Aperiodic Tilings

Yaroslav Don and Eric Akkermans
*Department of Physics, Technion – Israel Institute of Technology, Haifa 3200003, Israel*

## Appendix A: Cut and Project

In this appendix, we show how to make periodic and quasiperiodic structures using the C&P scheme.

### 1. The Procedure

The canonical C&P procedure is as follows [1].

**Cut:**

1. Start with an $n$-dimensional space $R = \mathbb{R}^n$.
2. Insert "atoms" on the integer lattice $Z = \mathbb{Z}^n$.
3. Divide $R$ into the *physical space* $E_\parallel$ and the *internal space* $E_\perp$ such that $E_\parallel \oplus E_\perp = R$ and $E_\parallel \cap E_\perp = \emptyset$.
4. To resolve ambiguity for $E_\parallel$, choose an initial location $\boldsymbol{c} \in R$ such that $E_\parallel$ passes through $\boldsymbol{c}$. There is no such requirement for $E_\perp$.

**Project:**

1. Inspect the hypercube $\mathbb{I}_n = [-0.5, 0.5)^n$.
2. The *window* is its projection on the internal space $W = \pi_\perp(\mathbb{I}_n)$.
3. The *strip* is the product with the physical space $S = W \otimes E_\parallel$.
4. Choose only the points inside the strip $S \cap Z$, and project them onto the physical space, $Y = \pi_\parallel(S \cap Z)$.
5. The *atomic density* is given by $\rho(\boldsymbol{x}) \equiv \rho_{\boldsymbol{c}}(\boldsymbol{x}) = \sum_{\boldsymbol{y}\in Y} \delta(\boldsymbol{x} - \boldsymbol{y})$ with $\boldsymbol{x} \in E_\parallel$. Note the implicit dependency of $Y$ on $\boldsymbol{c}$.

The C&P for $2D \to 1D$ is given in Fig. A1. Here, there are only 2 possible distances between neighboring atoms, $l_A, l_B$. This gives us the notion of a *tiling* of the letters $A$ and $B$. Another way to create this tiling is by moving in a stairway fashion on the atoms inside the strip: assign $A$ to a rightwards movement and $B$ to the upward one.

### 2. Rational Approximations by Continued Fractions

In order to work with finite systems $w_N$, a proper approximation method is needed for the infinite quasiperiodic system. We suggest approximating the slope $s$ by the continued fraction

$$s = a_0 + \cfrac{1}{a_1 + \frac{1}{a_2 + \frac{1}{a_3 + \dots}}} = [a_0; a_1, a_2, a_3, \dots], \tag{A1}$$

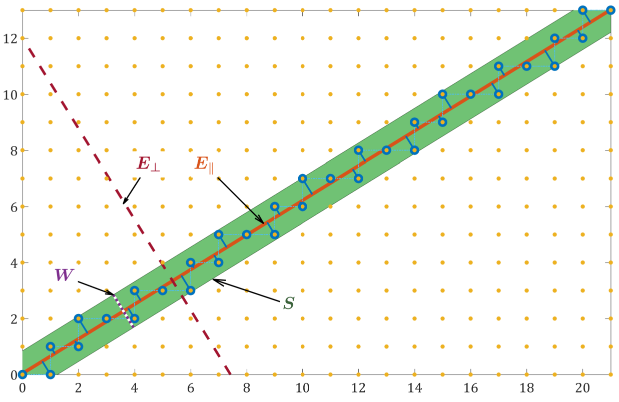


Figure A1. The cut and project scheme.

where $a_0 \in \mathbb{Z}$ is an integer and $a_{i\geq 1} \in \mathbb{N}$ natural numbers. Setting the approximation $s_N = [a_0; a_1, a_2, a_3, \dots, a_N]$, one has $s_N \to s$ as $N \to \infty$. Additionally, we obtain the sequence of numerators and denominators $s_N = c_N/d_N$. The denominators $d_N$ set the length of the word for the $N$-th approximation; the numerators $c_N$ relate them to the phason $\phi$ as described in the main text. We call $w_N$ the finite approximation to $w_\infty$.

Using finite approximants of continued fractions is not only convenient but of crucial importance. The ideas of the phases presented below work only for finite structures of size $d_N$. So does the correspondence between all C&P models (the canonical, $\Sigma_1$ and the characteristic function). We state that continued fractions exhibit the optimal approximation in due to the following inequality,

$$\left| s - \frac{c_N}{d_N} \right| < \frac{1}{d_N^2}. \tag{A2}$$

In other words, it is the best rational approximation for any denominators smaller than $d_N$.

## Appendix B: Gap Labeling Theorem

In this appendix, we present succinctly how to calculate the gap labels according to the gap labeling theorem.

### 1. Gap Labeling Formula

For a $1D$ substitution $\sigma$ with occurrence matrix $M$, the possible gaps in the spectrum are given by [2]

$$\mathcal{N}_{\text{gap}} = \frac{1}{a}\frac{k}{\lambda_*^N} \pmod 1, \quad a, k, N \in \mathbb{N}. \tag{B1}$$

Here, $\lambda_*$ is the leading (largest) eigenvalue of $M$. The calculation of the normalization factor $a$ is given below. For $d = \det(M) \neq 0$, this can be rewritten as

$$\mathcal{N}_{\text{gap}} = \frac{1}{a}\frac{p + q/\lambda_*}{d^N} \pmod 1, \quad p, q \in \mathbb{Z}. \tag{B2}$$

For a $1D$ C&P tiling with slope $s$, the possible gaps are given by

$$\mathcal{N}_{\text{gap}} = p + qs \pmod 1, \quad p, q \in \mathbb{Z}. \tag{B3}$$

### 2. Calculation of the Normalization Factor

Let us introduce letter doublets $L_k = l_i l_j$, where $l_i l_j$ are all *possible neighbors* in $w_\infty$. We then rewrite $w_\infty$ in terms of $L_k$ denoting it $w_\infty^2$. We denote the set of all doublets as $\Gamma_2 = \{L_k\} = \{\alpha, \beta, \gamma, \ldots\}$ .

The next step to define a substitution $\sigma_2 : \Gamma_2 \to \Gamma_2^{\mathbb{N}}$. It is done as follows for each letter $L \in \Gamma_2$ [3].

(a) Translate back to $L = l_1 l_2 \ldots l_m$ where $l_i \in \Gamma_1$;

(b) Apply $\sigma(L) = \sigma(l_1 l_2 \ldots l_m) = \ell_1 \ell_2 \ldots \ell_n$;

(c) Calculate the length $d = |\sigma(l_1)|$;

(d) Define $S = \ell_1 \ell_2 \ldots \ell_{d+1}$;

(e) Translate $S = L_1 \ldots L_d$ in terms of $\Gamma_2$.

Then, the definition of $\sigma_2$ reads

$$\sigma_2(L) = S, \quad \forall L \in \Gamma_2. \tag{B4}$$

We then define the occurrence matrix $M_2$ similarly to $M$. The eigenvalues of $M_2$ contain all eigenvalues of $M$. Specifically, they have the same leading eigenvalue $\lambda_*$.

Next, calculate $a$ as follows. Take the respective leading left-eigenvectors $\boldsymbol{v}_*^L$ and $\boldsymbol{v}_{*,2}^L$. Inspect all their entries $v_i$. The least common multiplier of all $v_i$ (removing factors of $\lambda_*$) is $a^{-1}$.

For example, in the Fibonacci substitution, $\Gamma_1 = \{A, B\}$ and $\sigma(A) = AB$, $\sigma(B) = A$, one finds that $\Gamma_2 = \{\alpha = AA, \beta = AB, \gamma = BA\}$. Using the algorithm above, we obtain

$$\sigma_2^{\text{Fib}} : \begin{cases} \alpha \mapsto \beta\gamma, \\ \beta \mapsto \beta\gamma, \\ \gamma \mapsto \alpha; \end{cases} \tag{B5}$$

with the occurrence matrix

$$M_2^{\text{Fib}} = \begin{pmatrix} 0 & 1 & 1 \\ 0 & 1 & 1 \\ 1 & 0 & 0 \end{pmatrix}. \tag{B6}$$

Additionally, $\lambda_*^{\text{Fib}} = (\sqrt{5}+1)/2$ and $a_{\text{Fib}} = 1$.

### 3. Primitivity Condition

The primitivity of $M$ and $M_2$ ensures that

(a) the leading eigenvalue $\lambda_*$ is unique, real and positive;

(b) the leading eigenvectors $\boldsymbol{v}_*^L$ and $\boldsymbol{v}_{*,2}^L$ have strictly positive entries $v_i$ [4, 5].

These $v_i$ are interpreted as corresponding letter $l_i$ frequency in the infinite word $w_\infty$ [6]. They are used as probability measures in the calculation of GLT [2]. The Perron-Frobenius theorem above also holds for a general non-strictly-upper-triangular nonnegative matrix $M$ (see Thm. 2.20 in [4]) up to the uniqueness of $\lambda_*$.

## Appendix C: Čech Cohomology and $\zeta$-function

The natural topological group associated with tilings is the Čech cohomology [7]. Its exact definition is beyond the scope of this paper (see [8] for an introduction). Nonetheless, we show in this section how to calculate the groups $\check{H}^0$ and $\check{H}^1$ with integer coefficients.

### 1. Bratteli Diagrams

In this section, we show how to construct the Bratteli diagrams [7, 8]. We use the Fibonacci substitution $A \mapsto AB$, $B \mapsto A$ as an illustrative example.

Consider the shift-map $\gamma_n : \Gamma_n \to \Gamma_n$ defined by

$$\gamma_n(w_i) = w_j \quad \text{if } w_j \text{ follows } w_i \text{ in } w_\infty. \tag{C1}$$

The graphical representation of $\gamma_n$ is a Bratteli diagram $G_n$. Its nodes are in $\Gamma_n$ and edges are in $\Gamma_{n+1}$. For Fibonacci, the first few diagrams are

$G_0^{\text{Fib}} =$ 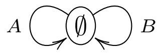 (C2a)


$G_1^{\text{Fib}} =$ 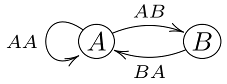 (C2b)


$G_2^{\text{Fib}} =$ 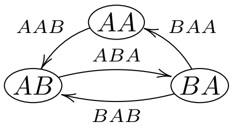 (C2c)


The zeroth diagram $G_0^{\text{Fib}}$ indicates that $w_\infty^{\text{Fib}}$ consists of $A$ and $B$ tiles. $G_1^{\text{Fib}}$ infers that $A$ is followed by either $A$ or $B$ in $w_\infty^{\text{Fib}}$, but $B$ is followed by $A$ only. This argument carries to $G_{n\geq 2}^{\text{Fib}}$. More diagrams are shown in Fig. C1.

Next, define the boundary operators on $G_n$ by

$$\partial_0(\alpha) = 0, \qquad \alpha, \beta \in \Gamma_n, \tag{C3a}$$

$$\partial_1(e) = \beta - \alpha, \qquad e = \overline{\alpha\beta} \in \Gamma_{n+1}. \tag{C3b}$$

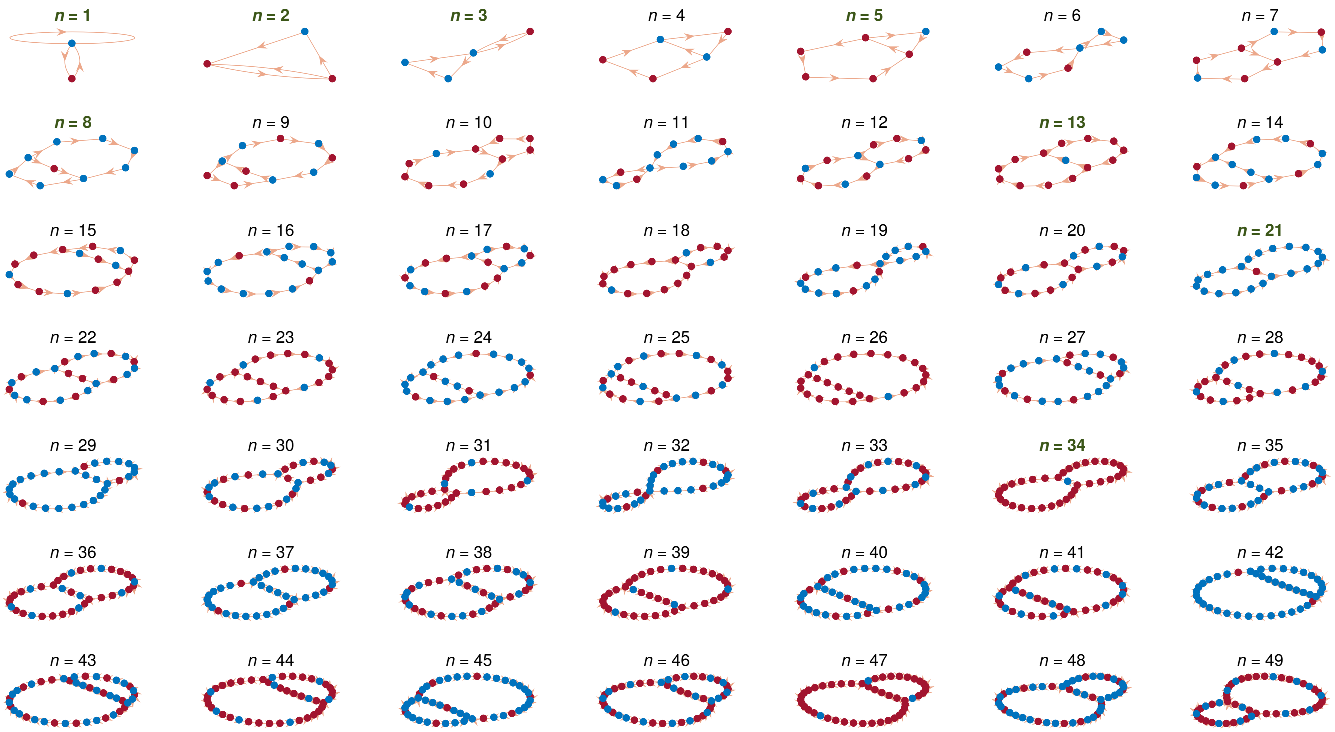


Figure C1. Bratteli diagrams for $n = 1 \dots 49$ of the C&P Fibonacci tiling with $s = \tau^{-2}$ and $\tau = (\sqrt{5}+1)/2$. Green titles indicate $n = d_N$. Blue and red nodes indicate different families identified by $L_N(n)$, the number of $B$-tiles in each supertile of size $n$ (explicitly, $L_B^{I}(n) = \lfloor n \cdot s \rfloor$ for the blue nodes and $L_B^{II}(n) = \lceil n \cdot s \rceil$ for the red ones). Yellow arrows indicate the edges.

The $\partial_k$ operators are represented as matrices $|\Gamma_n| \times |\Gamma_{n+1}|$ over $\mathbb{Z}$. Define the coboundary by

$$\delta^k = \partial_k^{\mathsf{T}}. \tag{C4}$$

Define the simplicial cohomology of a complex $G_n$ by

$$H_n^k = \frac{\ker \delta^k}{\operatorname{im} \delta^{k+1}} = \frac{\operatorname{coker} \partial_k}{\operatorname{coim} \partial_{k+1}}, \tag{C5}$$

where $(\operatorname{coker} d)$ $\ker d$ is the (co)kernel of $d$, and $(\operatorname{coim} d)$ $\operatorname{im} d$ is its (co)image.

### 2. Čech Cohomology Calculation

The Čech cohomology is formally defined as the inverse limit of all $H_n^k$

$$\check{H}^k = \varprojlim H_n^k. \tag{C6}$$

The exact definition of this limit appears in [7, 8]. To calculate $\check{H}^k$, we apply $\sigma$ on $G_n$ as follows.

1) Apply $\sigma_{n+1}$ on the edges of $G_n$.
   - The calculation of $\sigma_n$ is a generalization of the procedure in Appendix B2 from $\Gamma_2$ to $\Gamma_n$. Explicitly, redefine $S = \ell_1 \ell_2 \dots \ell_{d+n-1}$ in step (d).
   - A slightly different version of $\sigma_n$ appears in [7, 8] based on "collared tiles". For $\sigma_3$, denote $e = |\sigma(l_2)|$ and set $S = \ell_d \ell_{d+1} \dots \ell_{d+e+1}$ in step (d).
2) Deduce the nodes as the heads and tails of relevant edges in $\sigma(G_n)$.
3) Compute the inflation matrices $A_0 : \Gamma_n \to \Gamma_n$ and $A_1 : \Gamma_{n+1} \to \Gamma_{n+1}$ by identifying the transformation of the nodes and edges, respectively.

To calculate $\check{H}^k$, compute $A_0$ and $A_1$ of $G_2$ (though $G_0$ may also work in some cases). In Fibonacci,

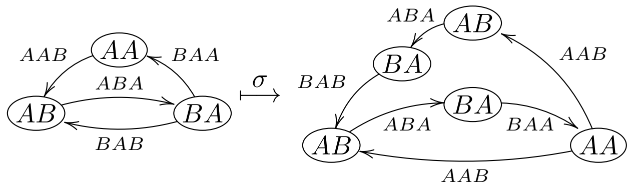


(C7)

Inspecting the nodes, $AA \to AB$, $AB \to AB$ and $BA \to AA$ (ignoring all the extra nodes in $\sigma(G_2)$). For the edges, $\overline{AAB} \to \overline{ABA}\,\overline{BAB}$, and so on. Summarizing, we arrive to $A_0$ and $A_1$ as follows

$$A_1^{\mathsf{T}} = \begin{pmatrix} 0 & 1 & 0 & 1 \\ 0 & 1 & 1 & 0 \\ 1 & 0 & 0 & 0 \\ 1 & 0 & 0 & 0 \end{pmatrix}, \quad A_0^{\mathsf{T}} = \begin{pmatrix} 0 & 1 & 0 \\ 0 & 1 & 0 \\ 1 & 0 & 0 \end{pmatrix}. \tag{C8}$$

With the inflation matrices $A_0$ and $A_1$, the $\zeta$-function is given by [7]

$$\zeta(z) = \frac{\det\left(I - zA_0^{\intercal}\right)}{\det\left(I - zA_1^{\intercal}\right)} = \frac{p_0(z)}{p_1(z)}. \tag{C9}$$

The Čech cohomology can be deduced from $p_m(z)$ by decomposing it to its irreducible components over the integers [9]. Namely, if

$$p_k(z) = \prod_{i=1}^{I}(1 - c_i z)\prod_{j=1}^{J}\left(1 - d_j z - e_j z^2\right), \tag{C10}$$

with $c_i, d_j, e_j \in \mathbb{Z}$, then

$$\begin{aligned}\check{H}^k \cong\ & \mathbb{Z}\left[c_1^{-1}\right] \oplus \cdots \oplus \mathbb{Z}\left[c_I^{-1}\right] \\ & \oplus \mathbb{Z}^2\left[e_1^{-1}\right] \oplus \cdots \oplus \mathbb{Z}^2\left[e_J^{-1}\right],\end{aligned} \tag{C11}$$

with $\mathbb{Z}[1/c] = \{n/c^m \mid n, m \in \mathbb{Z}\}$. Irreducible polynomials of higher orders are naturally generalized.

For example, in Fibonacci,

$$\zeta_{\text{Fib}}(z) = \frac{1 - z}{1 - z - z^2}. \tag{C12}$$

The numerator is trivial; the denominator has 2 irrational roots. Hence,

$$\check{H}^0_{\text{Fib}} \cong \mathbb{Z}, \tag{C13a}$$
$$\check{H}^1_{\text{Fib}} \cong \mathbb{Z}^2. \tag{C13b}$$

Generally, in any tiling space, $\check{H}^0 \cong \mathbb{Z}$ implying the tiling space is connected. Notice that if $\deg p_1 < |\Gamma_1|$, it implies one of the $c_i = 0$ in $p_1$. Therefore, (C13) is no longer valid. These are periodic substitutions; we therefore set $\check{H}^1 \cong \mathbb{Z}$ in this case.

The above procedure is for $1D$ tilings. In $2D$ tilings, the calculation of $\check{H}^0$, $\check{H}^1$ and also $\check{H}^2$ is more convoluted, and $\zeta(z)$ is not sufficient. The exact details appear in [7, 8].

### 3. Complexity

Define the *complexity* by the number of *nodes* in each complex [10]

$$c_n = |\Gamma_n|. \tag{C14}$$

Now, inspect the projection maps $\pi_n : \Gamma_{n+1} \to \Gamma_n$ between the complexes

$$\Gamma_0 \xleftarrow{\pi_0} \Gamma_1 \xleftarrow{\pi_1} \Gamma_2 \xleftarrow{\pi_2} \Gamma_3 \xleftarrow{\pi_3} \ldots \tag{C15}$$

which act by omitting the last letter in $\Gamma_{n+1}$.

There is a well-defined inverse limit [8]

$$\Omega = \varprojlim \Gamma_n. \tag{C16}$$

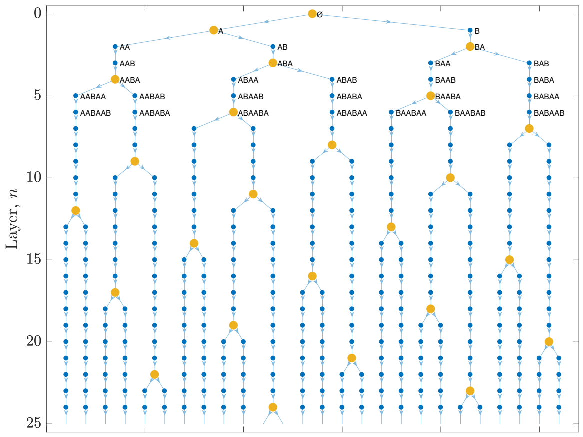


Figure C2. The complexity graph for the Fibonacci tiling. The arrows represent the mapping $\gamma_n$. In blue, the $n$-nodes ($n$-letter words) for each level (row) $n$, and in yellow – the $n$-nodes that split by $\gamma_n$ into two $(n+1)$-nodes. The total sum of splits at each row $n$ gives $s_n$. The first few nodes are labeled.

Here $\Omega$ is the tiling space to consider. Inspect the inverse maps $\pi_n^{-1}$, which give the options for the last adjacent letter to create $\Gamma_{n+1}$ from $\Gamma_n$. In other words, $\pi_n^{-1}$ correspond to the *edges* in the Bratteli diagram; thus

$$\pi_n^{-1} = \gamma_n. \tag{C17}$$

Hence, define the complexity tree $T_n$ by the sequence

$$T_n = \Gamma_0 \xrightarrow{\gamma_0} \Gamma_1 \xrightarrow{\gamma_1} \Gamma_2 \xrightarrow{\gamma_2} \ldots \xrightarrow{\gamma_{n-1}} \Gamma_n. \tag{C18}$$

This is seen in Fig. C2.

Consider the *splits* at each level $\Gamma_n$ as shown in Fig. C2. Here, $y_n$ is the number of nodes in level $n$ that have $> 1$ *outgoing* edges, and $s_n$ is the total number of splits. Note that for binary substitutions, $y_n = s_n$.

Now, since $\beta_n^1$ counts the number of cocycles in $\Gamma_n$ and the Bratteli graphs are connected ($\beta_n^0 = 1$ for all $n$), each split contributes an additional cocycle. Thus

$$\beta_n^1 = s_n + 1. \tag{C19}$$

Next, inspect the complexity $p(n) = c_n$, the total number of letters at level $n$. At each level $n$, $s_{n-1}$ letters are added to the letters of the $(n-1)$-th level; thus

$$c_n = s_{n-1} + c_{n-1}, \qquad c_0 = 1. \tag{C20}$$

Therefore,

$$c_n = 1 + \sum_{i=0}^{n-1} s_i. \tag{C21}$$

For C&P (Sturmian) sequences, where $\beta_n^1 = 2$ (equally, $s_n = 1$) for all $n$, one has $c_n = n + 1$. For primitive substitution tilings, the cohomology is bound, $\beta_n^1 \leq C+1$; thus $c_n \leq Cn + 1 = O(n)$ [10, 11]. For a periodic tiling, $\beta_{n>N}^1 = 1$ (equally, $s_{n>N} = 0$) for some $N \in \mathbb{Z}$; thus, the complexity is constant, $c_{n>N} = C$.

## Appendix D: Scattering Matrix Formalism

In this appendix, we present the spectral features of aperiodic structures. The avid reader is referred to [12, 13] for further details.

### 1. Transfer Matrix

We now present succinctly the main results of the transfer matrix in the wave equation. Consider a $1D$ system of size $L$ of some dielectric material. Its wave equation reads

$$-\psi''(x) - k_0^2\, v(x)\, \psi(x) = k_0^2\, \psi(x)\,. \tag{D1}$$

One has waves incoming to the system from the left and right, and outgoing waves after transmission and reflection. The free part (without dielectrics) has a well-defined $k$ vector, but the system itself need a more careful analysis. Next, consider scattering boundary conditions using $v(x) = \epsilon(x)/\bar{\epsilon} - 1 = n^2(x) - 1$ with $n(x)$ the refractive index [12]. We consider $v(x)$ build in the same quasiperiodic manner as above using $\Sigma_1$. In other words, we have $d_N$ slabs of refraction index $n_{A,B}$ and width $l_{A,B}$ so that $n_A l_A = n_B l_B$ ordered in a quasiperiodic way.

If we consider our system built of different dielectric media (width and permittivity), neglecting internal losses in the system, the total transfer matrix from left to right is written as

$$\begin{pmatrix}\psi_R^{\imath}\\ \psi_R^{\mathrm{o}}\end{pmatrix} = \mathcal{T}_W \begin{pmatrix}\psi_L^{\imath}\\ \psi_L^{\mathrm{o}}\end{pmatrix} = T_M \cdots T_2 T_1 \begin{pmatrix}\psi_L^{\imath}\\ \psi_L^{\mathrm{o}}\end{pmatrix}, \tag{D2}$$

and all the $T_m$-s are either propagation inside a slab or transfer between slabs as follows [12, 14]. For propagation one uses

$$T_A = \begin{pmatrix}\cos\delta_A & -\sin\delta_A\\ \sin\delta_A & \cos\delta_A\end{pmatrix}, \quad T_B = \begin{pmatrix}\cos\delta_B & -\sin\delta_B\\ \sin\delta_B & \cos\delta_B\end{pmatrix}, \tag{D3}$$

where the optical path is given by $\delta_A(k) = k n_A l_A$ with $k$ the wavevector, $n_A$ the refraction index of the slab of type $A$ and $l_A$ its width (similarly for $\delta_B$). To simplify the calculations, one uses the same optical path $\delta_A(k) = \delta_B(k) = \delta(k)$, so that

$$n_A l_A = n_B l_B. \tag{D4}$$

For the interface between slabs one uses

$$T_{A\to B} = \begin{pmatrix}1 & 0\\ 0 & n_B/n_A\end{pmatrix}, \quad T_{B\to A} = \begin{pmatrix}1 & 0\\ 0 & n_A/n_B\end{pmatrix}. \tag{D5}$$

### 2. Scattering Matrix

Take the structure of slabs and perform a scattering experiment. The scattering $\mathcal{S}$-matrix is defined by

$$\begin{pmatrix}\vec{o}\\ \overleftarrow{o}\end{pmatrix} = \begin{pmatrix}\vec{r}(k) & t(k)\\ t(k) & \overleftarrow{r}(k)\end{pmatrix}\begin{pmatrix}\vec{\imath}\\ \overleftarrow{\imath}\end{pmatrix} = \mathcal{S}\begin{pmatrix}\vec{\imath}\\ \overleftarrow{\imath}\end{pmatrix}, \tag{D6}$$

with $\vec{r} = r\exp(\mathrm{i}\vec{\vartheta})$ and $\overleftarrow{r} = r\exp(\mathrm{i}\overleftarrow{\vartheta})$ the rightwards and leftwards reflection coefficients and $t$ is the transmission coefficient. There is a well-defined procedure to translate $\mathcal{T}$ to $\mathcal{S}$ (see [12, 15]). For $\mathcal{T}(k) = \begin{pmatrix}M_1(k) & M_3(k)\\ M_2(k) & M_4(k)\end{pmatrix}$, one has

$$\vec{r}(k) = \frac{(M_4 - M_1) + \mathrm{i}(M_2 + M_3)}{(M_1 + M_4) + \mathrm{i}(M_3 - M_2)}, \tag{D7a}$$

$$\overleftarrow{r}(k) = \frac{(M_1 - M_4) + \mathrm{i}(M_2 + M_3)}{(M_1 + M_4) + \mathrm{i}(M_3 - M_2)}, \tag{D7b}$$

$$t(k) = \frac{2}{(M_1 + M_4) + \mathrm{i}(M_3 - M_2)}. \tag{D7c}$$

The $\mathcal{S}$-matrix is unitary and thus can be diagonalized to $\mathcal{S} \mapsto \operatorname{diag}\begin{pmatrix}\mathrm{e}^{\mathrm{i}\gamma_1} & \mathrm{e}^{\mathrm{i}\gamma_2}\end{pmatrix}$ so that $\det\mathcal{S} = \mathrm{e}^{2\mathrm{i}\delta(k)}$ is identified with the total phase shift

$$\begin{aligned}2\,\delta(k) &= \gamma_1(k,\phi) + \gamma_2(k,\phi)\\ &= \operatorname{Im}\log\det\mathcal{S}(k,\phi)\,,\end{aligned} \tag{D8}$$

independent of $\phi$ with $\operatorname{Im}(z)$ the imaginary part of $z$. The Krein-Schwinger formula [12] allows to relate the change of density of states to the scattering data

$$\varrho(k) - \varrho_0(k) = \frac{1}{2\pi}\operatorname{Im}\frac{\mathrm{d}}{\mathrm{d}k}\log\det\mathcal{S}(k)\,, \tag{D9}$$

where $\varrho_0(k)$ is the free density of states (i.e. without the system). The integrated density of states is, therefore,

$$\mathcal{N}(k) - \mathcal{N}_0(k) = \delta(k)/\pi. \tag{D10}$$

The chiral phase expresses the directionality of the $\mathcal{S}$-matrix. It is defined by [14]

$$\Theta_s(k,\phi) = \vec{\vartheta}(k,\phi) - \overleftarrow{\vartheta}(k,\phi)\,, \tag{D11}$$

which is $\phi$-dependent. Inside the gaps, $r = 1$ and $t = 0$; thus, the $\mathcal{S}$-matrix is diagonal, and we can identify $\gamma_1 = \vec{\vartheta}$ and $\gamma_2 = \overleftarrow{\vartheta}$. Therefore, $\Theta_s$ can be written as [9]

$$\Theta_s(k,\phi) = \operatorname{Im}\operatorname{Tr}\left[\sigma_z \log\mathcal{S}(k,\phi)\right], \tag{D12}$$

where $\sigma_z = \operatorname{diag}\begin{pmatrix}1 & -1\end{pmatrix}$ is the Pauli matrix.


[1] M. Duneau and A. Katz, Phys. Rev. Lett. **54**, 2688 (1985).

[2] J. Bellissard, A. Bovier, and J.-M. Ghez, Rev. Math. Phys. **04**, 1 (1992).

[3] M. Queffélec, *Substitution Dynamical Systems – Spectral Analysis*, 2nd ed., Lecture Notes in Mathematics, Vol. 1294 (Springer Berlin Heidelberg, 2010).

[4] R. S. Varga, *Matrix Iterative Analysis*, 2nd ed. (Springer Berlin Heidelberg, 2000).

[5] E. Seneta, *Non-negative Matrices and Markov Chains*, Rev. Print. ed., Springer series in statistics (Springer New York, 2006).

[6] J. M. Luck, C. Godrèche, A. Janner, and T. Janssen, J. Phys. A **26**, 1951 (1993).

[7] J. E. Anderson and I. F. Putnam, Ergod. Th. Dynam. Sys. **18**, 509 (1998).

[8] L. A. Sadun, *Topology of Tiling Spaces*, University Lecture Series, Vol. 46 (American Mathematical Society, 2008).

[9] Y. Don, *Topological Properties of Aperiodic Tilings and Fractals*, PhD Thesis, Technion – Israel Institute of Technology (2021).

[10] A. Julien, Ergod. Th. Dynam. Sys. **30**, 489 (2009).

[11] E. Arthur Robinson, Jr., in *Symbolic dynamics and its applications*, Proceedings of Symposia in Applied Mathematics, Vol. 60, edited by S. Williams (American Mathematical Society, 2004) pp. 81–120.

[12] E. Akkermans, G. V. Dunne, and E. Levy, in *Optics of Aperiodic Structures: Fundamentals and Device Applications*, edited by L. Dal Negro (Pan Stanford Publishing, 2013) pp. 407–449.

[13] E. Akkermans and G. Montambaux, *Mesoscopic Physics of Electrons and Photons* (Cambridge University Press, 2011).

[14] E. Levy, *Topological properties of quasiperiodic chains: structural and spectral analysis*, PhD Thesis, Technion – Israel Institute of Technology (2016).

[15] E. Levy and E. Akkermans, Eur. Phys. J. Special Topics **226**, 1563 (2017).
